# Supplementary material for: The Stacking in Bulk and Bilayer Hexagonal Boron Nitride
Source: arXiv:1307.0627 source file (2013-07-02)
Supplement: Supplementary file 1 [file Final_SI_a.pdf]

# The Stacking in Bulk and Bilayer Hexagonal Boron Nitride
# Supporting Informations

Gabriel Constantinescu, Agnieszka Kuc,* and Thomas Heine†
*School of Engineering and Science, Jacobs University Bremen,*
*Campus Ring 1, 28759 Bremen, Germany*

(Dated:)

TABLE S1. Calculated lattice parameters (in Å) at the DFT (DFT-D) and LMP2 levels of theory (including BSSE correction) for the bulk and the bilayer *h*-BN forms.

| **Method** | **bulk** | | **bilayer** | |
|---|---|---|---|---|
| | *a* | *c* | *a* | *c* |
| **BLYP(-D)** | 2.522 (2.512) | 5.494 (3.077) | 2.518 (2.517) | 5.493 (3.179) |
| **B3LYP(-D)** | 2.502 (2.496) | 4.333 (3.045) | 2.502 (2.501) | 4.334 (3.085) |
| **PBE(-D)** | 2.511 (2.506) | 4.126 (2.972) | 2.511 (2.517) | 4.176 (3.127) |
| **PBE0(-D)** | 2.494 (2.489) | 3.813 (2.956) | 2.494 (2.493) | 3.813 (2.987) |
| **PBEsol(-D)** | 2.504 (2.498) | 3.331 (2.884) | 2.503 (2.501) | 3.379 (2.924) |
| **LMP2** | 2.495 | 3.340 | 2.495 | 3.340 |
| **Exp.** | 2.504[1] | 3.330[1] | 2.510[2] | 3.25±0.10[2] |

At the PBE level, we have obtained *a* lattice parameter of 2.51 Å with perfect agreement to the results of Rydberg et al.[3] and Ribeiro et al.[4] at the same level. There have been a large number of LDA-based calculations reported in the literature and the *a* values obtained as this level vary from 2.48 Åto 2.50 Å.[5, 6] Subsequently, we have optimized the interlayer distance *c* of the AA' stacking fault in both bulk and bilayer forms. The dispersion corrected *c* values reported in the literature at the PBE(-D) level are 4.17 Å (3.33 Å) and 4.22 Å (3.37 Å),[7] in a close agreement with our results of 4.126 Å (2.972 Å) and 4.176 Å (3.127 Å), for the bulk and bilayer forms, respectively. Although our values are slightly lower than those of Marom et al.,[7] the relative difference between both bulk and bilayer forms is in a perfect agreement. Using PBE-D, Marini et al.[8] have obtained $c = 3.31$ Å for the *h*-BN bulk, while Rydberg et al.[3] have estimated much larger interlayer distance of 3.63 Å at the van der Waals corrected GGA level. Ribeiro et al.[4] have obtained the interlayer separation in the bilayer, at the PBE level, of 3.57 Å (AA' and AB), 3.60 Å (AB'), 3.72 Å (A'B), and 3.75 Å (AA)).

The energy sliding paths calculated using DFT(-D) methods show the same shapes, regardless of the density functional used, with the least stable stacking faults being the AA, A'B and AB' (in increasing order of stability). This is in agreement with other DFT calculations of Liu et al.[5] and Yin et al.[10] The authors have estimated the same trends between the least stable stacking orderings using LDA. Ooi et al.[11] have calculated the relative energy stabilities of various stacking faults in *h*-BN bulk using PBE, PW91 and LDA functionals. Due to the accuracy of the methods provided by the authors (1 meV per atom), all results suggested that the AA' and the AB stacking orderings are equally stable with about 2 meV per atom difference to the AB' structure. DFT is not accurate enough to resolve the stability differences between the AA' and AB orderings.

DFT-(D) can correctly predict the stability order of the least stable stackings and fails to resolve the differences between the AA' and the AB high-stability forms. The only exception in the BLYP method, that predicts the AA form to be highly stable. This deviation is due

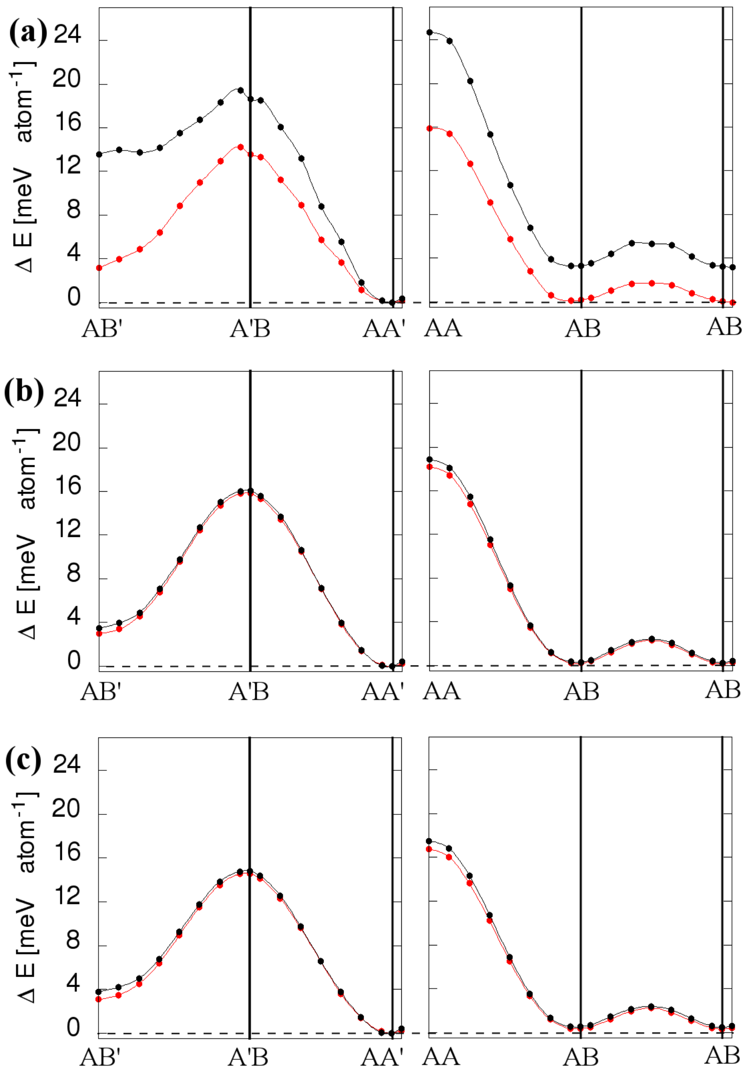


FIG. S1. BSSE-corrected (red) and uncorrected (black) energy sliding paths using BS1 (a), BS2 (b) and BS3 (c) basis sets (see text for details). All numbers are given with respect to the AA' stacking optimized at the DFT/PBEsol level. This functional gives the lattice parameters close to the experimental data independent of the basis set size: $a$ = 2.52 Å and $c$ = 6.69 Å for BS1, $a$ = 2.50 Å and $c$ =6.66 Å for BS2 and $a$ = 2.50 Å and $c$ = 6.66 Å for BS3.

to the very large optimized $c$ value (5.49 Å), that strongly exceeds even the reoptimized interlayer distances at the LMP2 level for this stacking ordering (3.62 Å).

To the best of our knowledge, however, stacking orderings other than AA' and AB have never been observed experimentally.

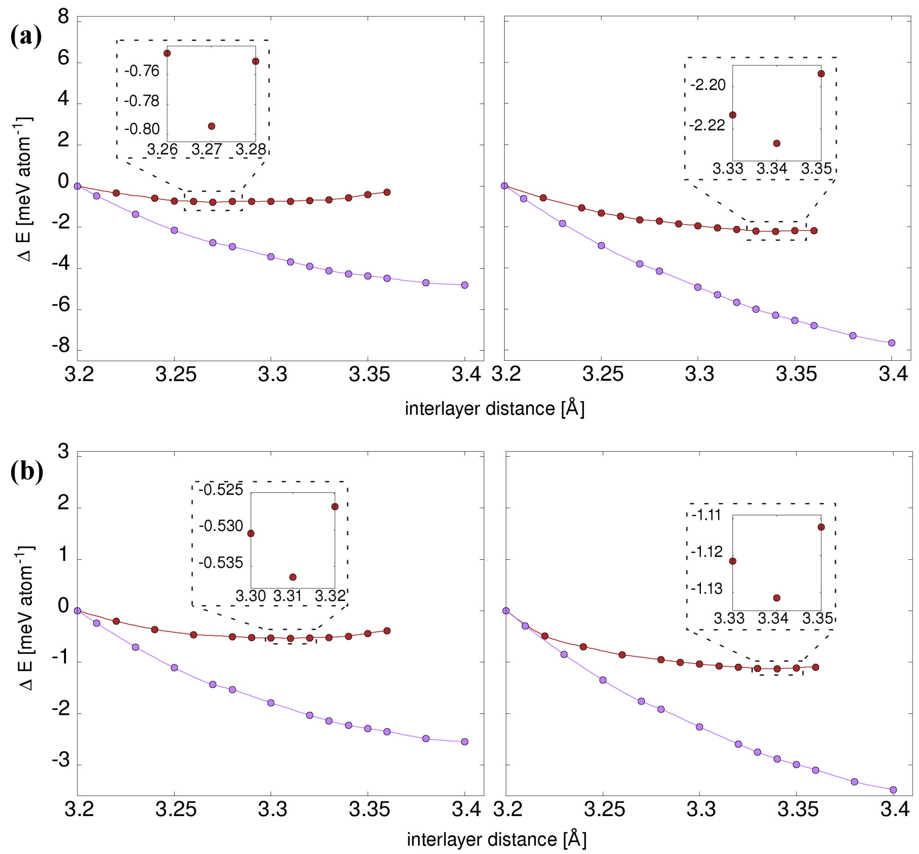


FIG. S2. Optimization of the interlayer distance $c$ in the AA' for of bulk (a) and bilayer (b) $h$-BN by means of LMP2 method.[9] Two larger basis sets were used: BS2 (purple) and BS3 (red). Left and right panels correspond to the BSSE uncorrected and corrected numbers, respectively. The insets show the zoom-in of the energy minima.

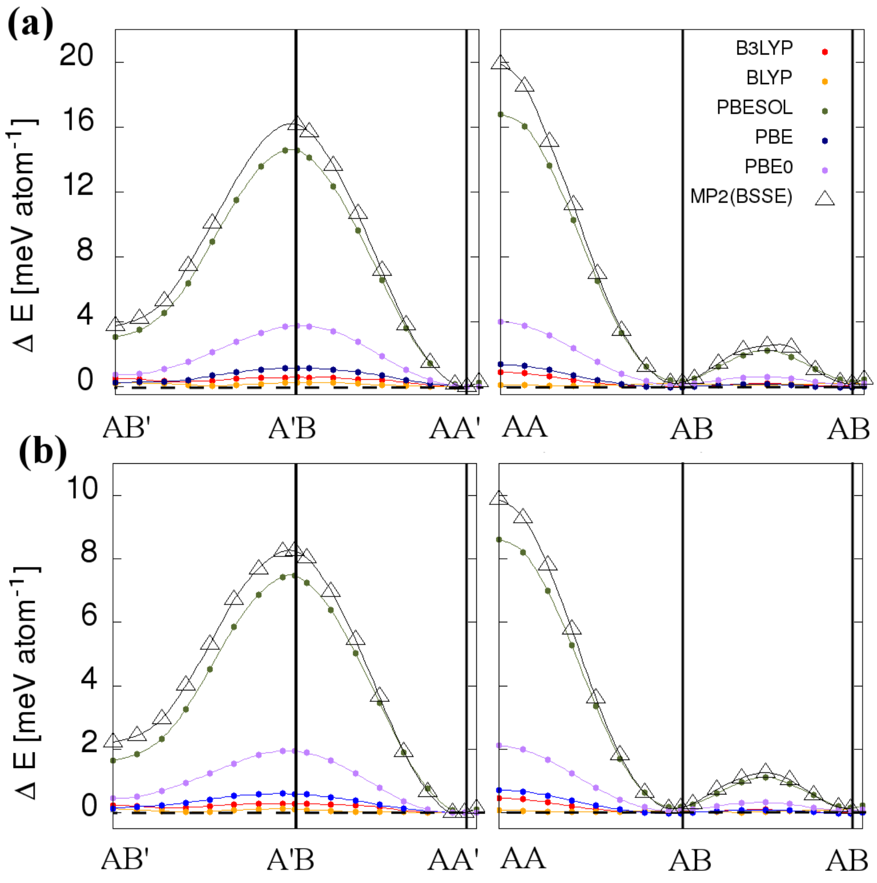


FIG. S3. BSSE-corrected energy sliding paths for the $h$-BN bulk (a) and bilayer (b) calculated using DFT methods with no dispersion correction. All numbers are given with respect to the AA' stacking.

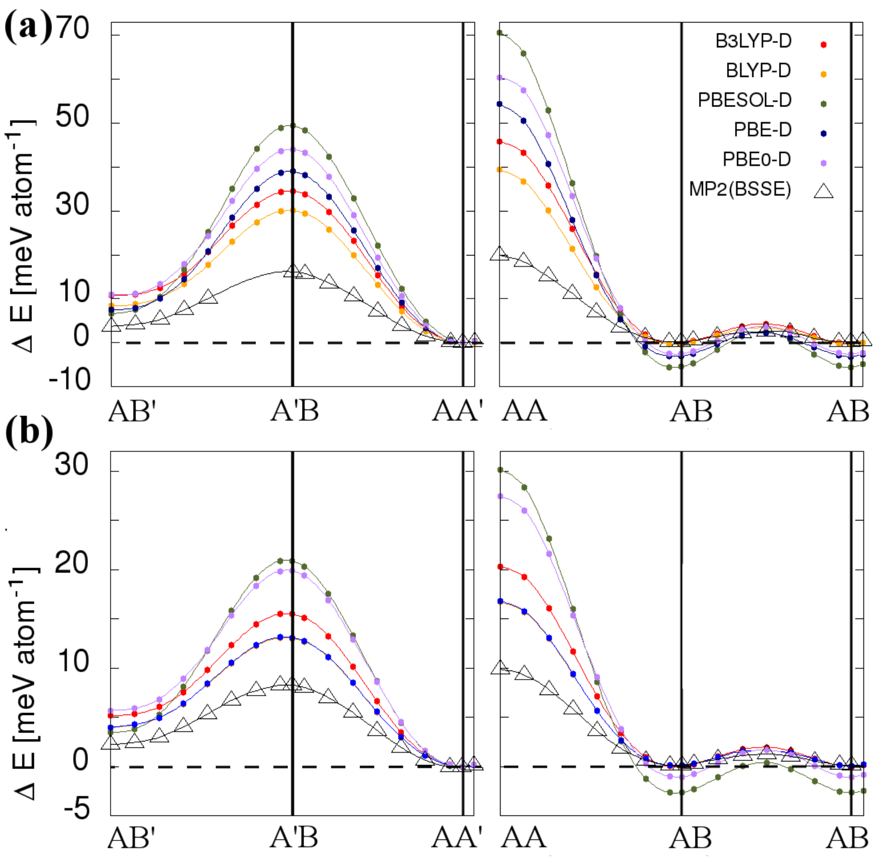


FIG. S4. BSSE-corrected energy sliding paths for the $h$-BN bulk (a) and bilayer (b) using DFT-D methods. All numbers are given with respect to the AA' stacking.

TABLE S2. Calculated relative energies of the high-symmetry stackings (in meV per atom) with the interlayer distances obtained using corresponding density functionals. All the numbers are given with respect to the AA' stacking.

| **Stacking** | **bulk** | | | | **bilayer** | | | |
|---|---|---|---|---|---|---|---|---|
| | A'B | AB' | AB | AA | A'B | AB' | AB | AA |
| **BLYP** | 0.25 | 0.21 | 0.19 | 0.11 | 0.11 | 0.13 | 0.09 | 0.09 |
| **BLYP-D** | 30.05 | 8.34 | -0.29 | 39.35 | 13.00 | 3.93 | 0.06 | 16.68 |
| **B3LYP** | 0.57 | 0.49 | 0.02 | 0.90 | 0.29 | 0.24 | 0.00 | 0.46 |
| **B3LYP-D** | 34.55 | 10.87 | -0.30 | 45.84 | 15.47 | 5.16 | -0.03 | 20.28 |
| **PBE** | 1.14 | 0.23 | -0.04 | 1.35 | 0.59 | 0.14 | -0.01 | 0.72 |
| **PBE-D** | 38.99 | 7.55 | -3.20 | 54.30 | 13.08 | 3.95 | 0.05 | 16.80 |
| **PBE0** | 3.75 | 0.74 | 0.10 | 4.01 | 1.94 | 0.45 | 0.06 | 2.12 |
| **PBE0-D** | 44.01 | 10.91 | -2.62 | 60.46 | 19.88 | 5.69 | -1.11 | 27.43 |
| **PBEsol** | 14.57 | 3.07 | 0.34 | 16.76 | 7.47 | 1.65 | 0.15 | 8.61 |
| **PBEsol-D** | 49.41 | 6.56 | -5.71 | 70.69 | 20.86 | 3.42 | -2.65 | 30.16 |

TABLE S3. Calculated relative energies of the high-symmetry stackings (in meV per atom) with the interlayer distance taken from the BSSE-corrected LMP2 results ($c = 3.34$Å). All the numbers are given with respect to the AA' stacking.

| **Stacking** | **bulk** | | | | **bilayer** | | | |
|---|---|---|---|---|---|---|---|---|
| | A'B | AB' | AB | AA | A'B | AB' | AB | AA |
| **BLYP** | 14.06 | 3.77 | 0.86 | 15.81 | 7.09 | 1.98 | 0.38 | 8.05 |
| **BLYP-D** | 14.09 | 4.12 | 0.93 | 16.04 | 7.10 | 2.16 | 0.42 | 8.16 |
| **B3LYP** | 15.48 | 4.72 | 1.22 | 17.55 | 7.85 | 2.51 | 0.54 | 8.97 |
| **B3LYP-D** | 15.51 | 5.08 | 1.20 | 17.78 | 7.86 | 2.68 | 0.56 | 9.09 |
| **PBE** | 13.84 | 2.80 | 0.30 | 15.84 | 7.04 | 1.52 | 0.13 | 8.11 |
| **PBE-D** | 13.87 | 3.15 | 0.38 | 16.06 | 7.06 | 1.70 | 0.17 | 8.23 |
| **PBE0** | 15.80 | 4.14 | 0.74 | 18.12 | 8.08 | 2.26 | 0.38 | 9.32 |
| **PBE0-D** | 15.83 | 4.49 | 0.90 | 18.35 | 8.10 | 2.44 | 0.46 | 9.44 |
| **PBEsol** | 13.80 | 2.74 | 0.22 | 15.91 | 7.07 | 1.50 | 0.13 | 8.18 |
| **PBEsol-D** | 13.83 | 3.09 | 0.29 | 16.14 | 7.09 | 1.68 | 0.14 | 8.30 |

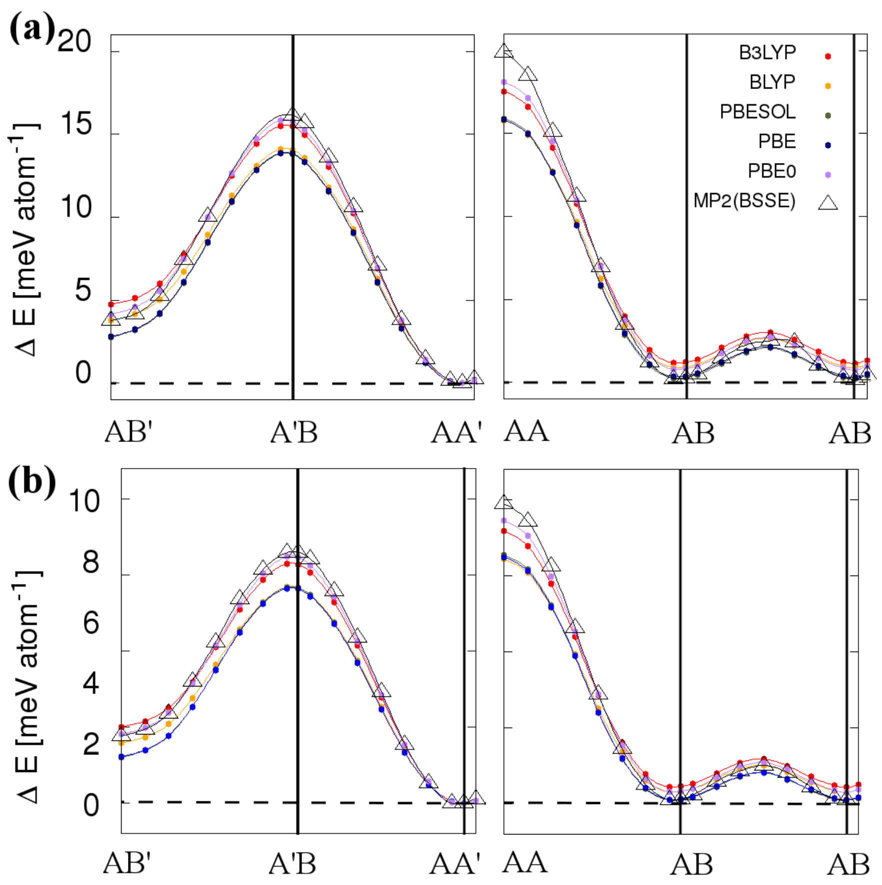


FIG. S5. BSSE-corrected energy sliding paths for the $h$-BN bulk (a) and bilayer (b) calculated using DFT methods with no dispersion correction. The interlayer distance is taken from the BSSE-corrected LMP2 results ($c = 3.34$Å). All numbers are given with respect to the AA' stacking.

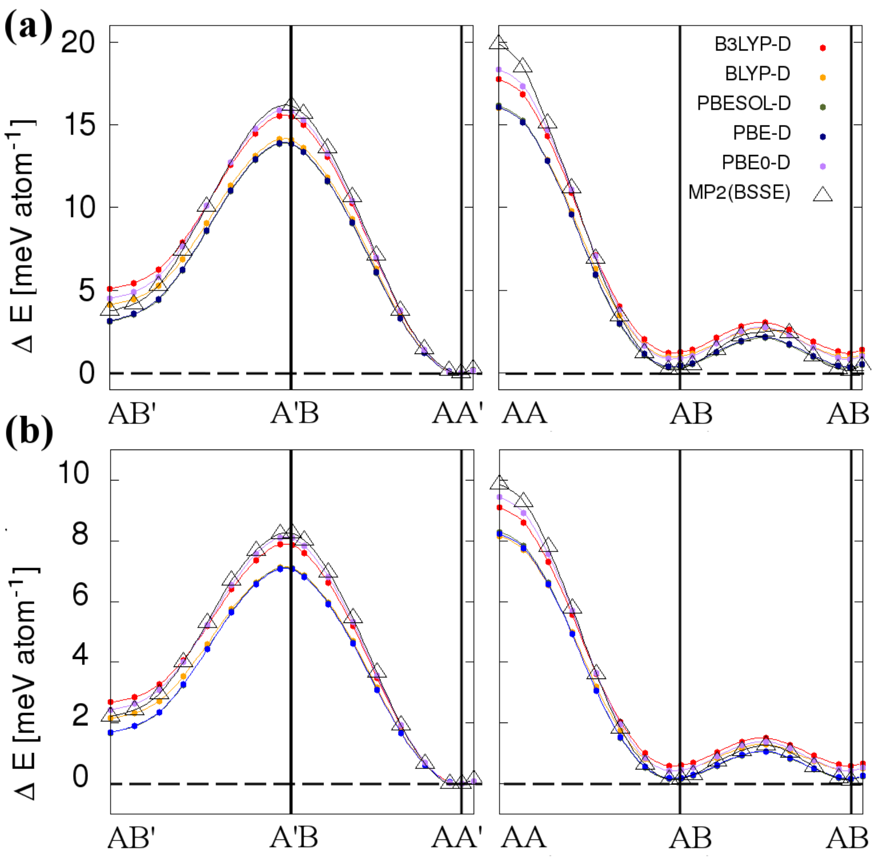


FIG. S6. BSSE-corrected energy sliding paths for the $h$-BN bulk (a) and bilayer (b) using DFT-D methods. The interlayer distance is taken from the BSSE-corrected LMP2 results. All numbers are given with respect to the AA' stacking.

* a.kuc@jacobs-university.de
† t.heine@jacobs-university.de
[1] Pease, R. S. *Nature* **1950**, *165*, 722–723.
[2] Warner, J. H.; Ruemmeli, M. H.; Bachmatiuk, A.; Buechner, B. *Acs Nano* **2010**, *4*, 1299–1304.
[3] Rydberg, H.; Dion, M.; Jacobson, N.; Schroder, E.; Hyldgaard, P.; Simak, S. I.; Langreth, D. C.; Lundqvist, B. I. *Physical Review Letters* **2003**, *91*, 126402–1–4.
[4] Ribeiro, R. M.; Peres, N. M. R. *Physical Review B* **2011**, *83*, 235312–1–6.
[5] Liu, L.; Feng, Y. P.; Shen, Z. X. *Physical Review B* **2003**, *68*, 104102–1–8.
[6] Mosuang, T. E.; Lowther, J. E. *Journal Of Physics And Chemistry Of Solids* **2002**, *63*, 363–368.
[7] Marom, N.; Bernstein, J.; Garel, J.; Tkatchenko, A.; Joselevich, E.; Kronik, L.; Hod, O. *Physical review letters* **2010**, *105*, 046801–1–4.
[8] Marini, A.; Garcia-Gonzalez, P.; Rubio, A. *Physical Review Letters* **2006**, *96*, 136404–1–4.
[9] Pisani, C.; Maschio, L.; Casassa, S.; Halo, M.; Schuetz, M.; Usvyat, D. *Journal of Computational Chemistry* **2008**, *29*, 2113–2124.
[10] Yin, J. L.; Hu, M. L.; Yu, Z.; Zhang, C. X.; Sun, L. Z.; Zhong, J. X. *Physica B-Condensed Matter* **2011**, *406*, 2293–2297.
[11] Ooi, N.; Rairkar, A.; Lindsley, L.; Adams, J. B. *Journal Of Physics-Condensed Matter* **2006**, *18*, 97–115.
